# Supplementary material for: WeaQA: Weak Supervision via Captions for Visual Question Answering
Source: arXiv:2012.02356 source file (2021-05-28)
Supplement: Supplementary file 1 [file supp_table_old.tex]

% \begin{table*}[t]
%     \centering
%     \resizebox{\textwidth}{!}
% {
%     \begin{tabular}{l>{\raggedright}p{50mm}>{\raggedright}p{25mm}>{\raggedright}p{50mm}p{25mm}}
%         \toprule
%         \textbf{Mutation} & $\mathbf{Q}$ & $\mathbf{A}$ & $\mathbf{Q_{new}}$ & $\mathbf{A_{new}}$ \\
%         \toprule
%         \multirow{4}{*}{Negation} & Is this bread? & yes & Is this not bread & no \\
%          & What is the color of the woman's shirt? & black & What is not the color of the woman's shirt? & white\\
%          & Are there deciduous trees? & no & Are there no deciduous trees? & yes \\
%          & Is there a boy? & no & Is there no boy? & yes \\
%         \midrule
%         \multirow{3}{*}{Adversarial} & Who is riding the boat? & man & Who is riding the desk & \textit{``can't say"}\\
%          & How big is the plane? & large & How big is the book? & \textit{``size"} \\
%          & How many pillows are on the bed? & four & How many pillows are on the table? & \textit{``number"} \\
        % \midrule 
        % \multirow{4}{*}{Paraphrasing} & How is something parked ? & illegally & How's-what's parked? & illegally\\
        %  & what does something seem to do ? & park & What do you think something seems to be doing? & park\\
        %  & Where was parked something? & behind a legally parked car & Do you know where something was parked? & behind a legally parked car \\
        %  & How many cars are visible ? & 2 & How many cars are we looking at? & 2 \\
        %  & Is there two cars parked on the sidewalk on the street ? & Yes & There are two cars parked on the sidewalk, right? & Yes \\
        %  & Is it a bathroom sink with toiletries on the counter ? & Yes & Is a washbasin with toiletries on counter? & Yes \\
        %  \midrule
        %   \multirow{4}{*}{Templates} & What are set on the sidewalk outside a veterinary hospital? & bags &  & \\
        %  & What is the young man holding up in front of his face ? & phone &  & \\
        %  & What is almost empty on the table & glass &  & \\
        %  & What drawn carriage with passengers in the city & horse &  &  \\
        %  & What is the color of the table ? & white &  &  \\
        %  & What is the color of the eyes ? & blue &  &  \\
        % %  & How many boats anchored by ropes close to shore? & 8 & & \\
    %     \bottomrule
    % \end{tabular}
    % }
    % \caption{Examples of three types of question transformation with corresponding answers}
    % \label{tab:negation}

% \end{table*}
